# Supplementary material for: Parameter Estimation for Scarce Stellar Populations
Source: arXiv:1904.09054 source file (2019-04-19)
Supplement: Supplementary file 1 [file appendix.tex]

\appendix\label{appen}

\section{}

\begin{figure*}

\includegraphics[scale= 0.55]{ramirez-siordia-et_al-fig2-Appendix.pdf}
\caption{
$\mathcal{L}_N^{cond}$ distributions for $t, m-M$, $E(B-V)$, and Z. 
Two different subsamples were defined for each UFDG by trimming the sample below the colour coded $m_{814}$ magnitude cuts shown in Fig.~\ref{fig7}.} 
\label{figA2}
\end{figure*}

\begin{table*}
\caption{Mock galaxy with 2 old stellar populations varying $w_y$}
\label{tab3Appendix}
\begin{tabular}{|c|c|c|c|c|c|c|}
\hline
$w_{y,true}$    & $w_{y,est}$     & $t_{o,est}$ (Gyr)     & $t_{y,est}$ (Gyr)      & $(m-M)_{est}$   & $E(V-I)_{est}$    & $Z_{est}$                       \\ \hline
0.1             & $\sim$0.15      & $12.0_{-1.2}^{+1.4}$  & $8.0_{-3.75}^{+3.0}$      & 21.9$\pm$0.2    & 0.09$\pm$0.03     & $0.0001 _{-0.00005}^{+0.00006}$ \\
0.3             & $\sim$0.45      & $12.0_{-1.2}^{+1.8}$  & $8.0_{-1.5}^{+1.8}$    & 21.9$\pm$0.2    & 0.09$\pm$0.03     & $0.0001 _{-0.00005}^{+0.00006}$ \\
0.5             & $\sim$0.55      & $12.0_{-1.7}^{+2.8}$  & 8.25$\pm$1.4           & 21.9$\pm$0.2    & 0.085$\pm$0.03    & $0.0001 _{-0.00005}^{+0.00008}$ \\
0.7             & $\sim$0.80      & $12.0_{-2.5}^{+3}$   & 8.0$\pm$1.1           & 21.9$\pm$0.2    & 0.09$\pm$0.03     & $0.0001 _{-0.00005}^{+0.00008}$ \\
0.9             & $\sim$0.95      & $12.0_{-4.0}^{+5}$     & 8.0$\pm$1.0           & 21.9$\pm$0.2    & 0.09$\pm$0.03     & $0.0001 _{-0.00005}^{+0.00009}$ \\ \hline
\end{tabular}
\end{table*}

\begin{table*}
\caption{Mock galaxy with 2 young stellar populations varying $w_y$}
\label{tab4Appendix}
\begin{tabular}{|l|l|l|l|l|l|l|}
\hline
$w_{y,true}$    & $w_{y,est}$  & $t_{o,est}$ (Myr) & $t_{y,est}$ (Myr)  & $(m-M)_{est}$     & $E(V-I)_{est}$ & $Z_{true}$ \\ \hline
0.1             &    &       & 6.0$\pm$0.2        & 29.00$\pm$0.12    & 0.15$\pm$0.02  & 0.008      \\
0.3             & $\sim$0.30   & 6.25$\pm$0.2      & 4.2$\pm$0.5        & 28.92$\pm$0.10    & 0.15$\pm$0.02  & 0.008      \\
0.5             & $\sim$0.50   & 6.0$\pm$0.3       & 4.1$\pm$0.3        & 29.01$\pm$0.11    & 0.15$\pm$0.02  & 0.008      \\
0.7             & $\sim$0.75   & 6.0$\pm$0.3       & 4.0$\pm$0.3        & 29.01$\pm$0.12    & 0.15$\pm$0.02  & 0.008      \\
0.9             & $\sim$0.90   & 6.0$\pm$0.7       & 4.1$\pm$0.3        & 29.01$\pm$0.20    & 0.15$\pm$0.02  & 0.008      \\ \hline
\end{tabular}
\end{table*}
